# Supplementary material for: Using Linear Dynamical Topic Model for Inferring Temporal Social Correlation in Latent Space
Source: arXiv:1501.01270 source file (2015-01-06)
Supplement: Supplementary file 1 [file appendices.tex]

\section*{APPENDIX}
\setcounter{section}{1}
\label{sec:appendix}

\begin{comment}
	\begin{pmatrix}
	\mu_{n,t,1} & \ldots & 0 & \ldots & 0 \\
	\vdots & \ddots & \vdots & \iddots  &  \vdots \\
	0 & \ldots & \mu_{n,t,k} & \ldots & 0 \\
	\vdots & \iddots & \vdots & \ddots & \vdots \\
	0 & \ldots & 0 & \ldots & \mu_{n,t,K} \\ 
	\end{pmatrix}
\end{comment}

\[ A_{n,t} = \begin{pmatrix} \mu_{n,t,1} & & \\ & \mu_{n,t,k} & \\ & & \mu_{n,t,K} \end{pmatrix} \]
Assume that the dynamics matrix $A_{n,t}$ is a diagonal matrix with entries $\{ \mu_{n,t,1},\ldots,\mu_{n,t,K} \}$. We express the individual components of Equation \ref{eqn:gradient_mu} from Section \ref{sec:estimate_dynamics}. The same equation is also shown here for easy reference:

{\small \[ \frac{d \mathcal{L}}{d \mu_{n,t-1,k}} = \frac{d E \left( \theta_{n,t,k|t} \right) }{d \mu_{n,t-1,k}} \left[ \log \frac{ E \left( \theta_{n,t,k|t} \right) } { E \left( \theta_{n,t,k|t-1} \right) } \right] + E \left( \theta_{n,t,k|t} \right) \left[ \frac{d \log E \left( \theta_{n,t,k|t} \right) }{d \mu_{n,t-1,k}} - \frac{d \log E \left( \theta_{n,t,k|t-1} \right) }{d \mu_{n,t-1,k}} \right] \] }

Use the following equations:
\begin{gather*}
	E \left( \theta_{n,t,k|t-1} \right) = \frac{ \mu_{n, t-1, k} \cdot x_{n,t-1,k|t-1} + \alpha }{ 1' A_{n, t-1} \cdot x_{n,t-1|t-1} + K \alpha } \quad
	E \left( \theta_{n,t,k|t} \right) = \frac{ \mu_{n, t-1, k} \cdot x_{n,t-1,k|t-1} + \psi_{n, t, k} + \alpha }{ 1' \left( A_{n, t-1} \cdot x_{n,t-1|t-1} + \psi_{n, t} \right) + K \alpha } \\
\end{gather*}
\begin{align*}
	\frac{d E \left( \theta_{n,t,k|t} \right) }{d \mu_{n,t-1,k}} &= \frac{ x_{n,t-1,k|t-1} \left( 1' \psi_{n, t} + K \alpha \right) - 1' x_{n,t-1|t-1} \left( \psi_{n, t, k} + \alpha \right) }{ \left[ 1' \left( A_{n, t-1} \cdot x_{n,t-1|t-1} + \psi_{n, t} \right) + K \alpha \right]^2 } \\
	\frac{d \log E \left( \theta_{n,t,k|t} \right) }{d \mu_{n,t-1,k}} &= \frac{1}{E \left( \theta_{n,t,k|t} \right)} \frac{d E \left( \theta_{n,t,k|t} \right) }{d \mu_{n,t-1,k}} \\
	\frac{d \log E \left( \theta_{n,t,k|t-1} \right) }{d \mu_{n,t-1,k}} &= \frac{x_{n,t-1,k|t-1}}{\mu_{n,t-1,k} \cdot x_{n,t-1,k|t-1} + \alpha} - \frac{1' x_{n,t-1|t-1}}{1' A_{n, t-1} \cdot x_{n,t-1|t-1} + K \alpha}
\end{align*}
